# Supplementary material for: The algebraic spin liquid in the SU(6) Heisenberg model on the kagome lattice
Source: arXiv:2407.09713 source file (2025-11-30)
Supplement: Supplementary file 1 [file appendix_triangle_Hsu.pdf]

# The algebraic spin liquid and dynamical structure factor of the SU(6) Heisenberg model on the kagome lattice


Dániel Vörös,[1,2,1] Kránitz Péter,[1,2] and Karlo Penc[2]

[1]*Department of Theoretical Physics, Institute of Physics, Budapest University of Technology and Economics, Műegyetem rakpart 3, H-1111 Budapest, Hungary*

[2]*Institute for Solid State Physics and Optics, Wigner Research Centre for Physics, H-1525 Budapest, P.O. Box 49, Hungary*



(Dated: January 31, 2024)



Abstract


## I. INTRODUCTION

### Appendix A: Hsu

$$\bar{n}_i^X = 1 - n_i^X \tag{A1}$$

$$\begin{aligned} \xi_{i,j} &= \langle \mathrm{FS} | c_i^\dagger c_j | \mathrm{FS} \rangle \\ \bar{\xi}_{i,j} &= \langle \mathrm{FS} | c_j c_i^\dagger | \mathrm{FS} \rangle = -\xi_{i,j} \end{aligned} \tag{A2}$$

$$\begin{aligned} AAA &= \langle n_1^A \bar{n}_1^B \dots \bar{n}_1^F n_2^A \bar{n}_2^B \dots \bar{n}_2^F n_3^A \bar{n}_3^B \dots \bar{n}_3^F \rangle \\ &= \langle n_1^A n_2^A n_3^A \rangle \langle \bar{n}_1^B \bar{n}_2^B \bar{n}_3^B \rangle \dots \langle \bar{n}_1^F \bar{n}_2^F \bar{n}_3^F \rangle \\ &= \begin{vmatrix} \nu_1^A & \xi_{1,2}^A & \xi_{1,3}^A \\ \xi_{2,1}^A & \nu_2^A & \xi_{2,3}^A \\ \xi_{3,1}^A & \xi_{3,2}^A & \nu_3^A \end{vmatrix} \times \begin{vmatrix} \bar{\nu}_1^B & \bar{\xi}_{1,2}^B & \bar{\xi}_{1,3}^B \\ \bar{\xi}_{2,1}^B & \bar{\nu}_2^B & \bar{\xi}_{2,3}^B \\ \bar{\xi}_{3,1}^B & \bar{\xi}_{3,2}^B & \bar{\nu}_3^B \end{vmatrix} \times \dots \times \begin{vmatrix} \bar{\nu}_1^F & \bar{\xi}_{1,2}^F & \bar{\xi}_{1,3}^F \\ \bar{\xi}_{2,1}^F & \bar{\nu}_2^F & \bar{\xi}_{2,3}^F \\ \bar{\xi}_{3,1}^F & \bar{\xi}_{3,2}^F & \bar{\nu}_3^F \end{vmatrix} \end{aligned} \tag{A3}$$

$$\begin{aligned} AAB &= \langle n_1^A \bar{n}_1^B \dots \bar{n}_1^F n_2^A \bar{n}_2^B \dots \bar{n}_2^F \bar{n}_3^A n_3^B \dots \bar{n}_3^F \rangle \\ &= \langle n_1^A n_2^A \bar{n}_3^A \rangle \langle \bar{n}_1^B \bar{n}_2^B n_3^B \rangle \dots \langle \bar{n}_1^F \bar{n}_2^F \bar{n}_3^F \rangle \\ &= \begin{vmatrix} \nu_1^A & \xi_{1,2}^A & \xi_{1,3}^A \\ \xi_{2,1}^A & \nu_2^A & \xi_{2,3}^A \\ \bar{\xi}_{3,1}^A & \bar{\xi}_{3,2}^A & \bar{\nu}_3^A \end{vmatrix} \times \begin{vmatrix} \bar{\nu}_1^B & \bar{\xi}_{1,2}^B & \bar{\xi}_{1,3}^B \\ \bar{\xi}_{2,1}^B & \bar{\nu}_2^B & \bar{\xi}_{2,3}^B \\ \xi_{3,1}^B & \xi_{3,2}^B & \nu_3^B \end{vmatrix} \times \dots \times \begin{vmatrix} \bar{\nu}_1^F & \bar{\xi}_{1,2}^F & \bar{\xi}_{1,3}^F \\ \bar{\xi}_{2,1}^F & \bar{\nu}_2^F & \bar{\xi}_{2,3}^F \\ \bar{\xi}_{3,1}^F & \bar{\xi}_{3,2}^F & \bar{\nu}_3^F \end{vmatrix} \end{aligned} \tag{A4}$$

$$\begin{aligned} ABC &= \langle n_1^A \bar{n}_1^B \bar{n}_1^C \dots \bar{n}_1^F \bar{n}_2^A n_2^B \bar{n}_2^C \dots \bar{n}_2^F \bar{n}_3^A \bar{n}_3^B n_3^C \dots \bar{n}_3^F \rangle \\ &= \langle n_1^A \bar{n}_2^A \bar{n}_3^A \rangle \langle \bar{n}_1^B n_2^B \bar{n}_3^B \rangle \langle \bar{n}_1^C \bar{n}_2^C n_3^C \rangle \dots \langle \bar{n}_1^F \bar{n}_2^F \bar{n}_3^F \rangle \\ &= \begin{vmatrix} \nu_1^A & \xi_{1,2}^A & \xi_{1,3}^A \\ \bar{\xi}_{2,1}^A & \bar{\nu}_2^A & \bar{\xi}_{2,3}^A \\ \bar{\xi}_{3,1}^A & \bar{\xi}_{3,2}^A & \bar{\nu}_3^A \end{vmatrix} \times \begin{vmatrix} \bar{\nu}_1^B & \bar{\xi}_{1,2}^B & \bar{\xi}_{1,3}^B \\ \xi_{2,1}^B & \nu_2^B & \xi_{2,3}^B \\ \bar{\xi}_{3,1}^B & \bar{\xi}_{3,2}^B & \bar{\nu}_3^B \end{vmatrix} \times \begin{vmatrix} \bar{\nu}_1^C & \bar{\xi}_{1,2}^C & \bar{\xi}_{1,3}^C \\ \bar{\xi}_{2,1}^C & \bar{\nu}_2^C & \bar{\xi}_{2,3}^C \\ \xi_{3,1}^C & \xi_{3,2}^C & \nu_3^C \end{vmatrix} \times \dots \times \begin{vmatrix} \bar{\nu}_1^F & \bar{\xi}_{1,2}^F & \bar{\xi}_{1,3}^F \\ \bar{\xi}_{2,1}^F & \bar{\nu}_2^F & \bar{\xi}_{2,3}^F \\ \bar{\xi}_{3,1}^F & \bar{\xi}_{3,2}^F & \bar{\nu}_3^F \end{vmatrix} \end{aligned} \tag{A5}$$

off diagonal:

$$P_{12} AAA = AAA \tag{A6}$$

$$P_{12} AAB = AAB \tag{A7}$$

$$
\begin{aligned}
P_{12}ABA &= \langle c_1^{B\dagger} c_2^{A\dagger} c_2^{B} c_1^{A} n_1^{A} \bar{n}_1^{B} \ldots \bar{n}_1^{F} \bar{n}_2^{A} n_2^{B} \ldots \bar{n}_2^{F} n_3^{A} \bar{n}_3^{B} \ldots \bar{n}_3^{F} \rangle \\
&= \langle c_1^{B\dagger} c_1^{A} n_1^{A} \bar{n}_1^{B} \ldots \bar{n}_1^{F} c_2^{A\dagger} c_2^{B} \bar{n}_2^{A} n_2^{B} \ldots \bar{n}_2^{F} n_3^{A} \bar{n}_3^{B} \ldots \bar{n}_3^{F} \rangle \\
&= -\langle c_1^{A} c_1^{B\dagger} \ldots \bar{n}_1^{F} c_2^{A\dagger} c_2^{B} \ldots \bar{n}_2^{F} n_3^{A} \bar{n}_3^{B} \ldots \bar{n}_3^{F} \rangle \\
&= \langle c_1^{A} c_2^{A\dagger} n_3^{A} \rangle \langle c_1^{B\dagger} c_2^{B} \bar{n}_3^{B} \rangle \ldots \langle \bar{n}_1^{F} \bar{n}_2^{F} \bar{n}_3^{F} \rangle \\
&= \begin{vmatrix} \bar{\xi}_{1,2}^{A} & \bar{\xi}_{1,3}^{A} \\ \xi_{2,3}^{A} & \nu_3^{A} \end{vmatrix} \times \begin{vmatrix} \xi_{1,2}^{B} & \xi_{1,3}^{B} \\ \bar{\xi}_{2,3}^{B} & \bar{\nu}_3^{B} \end{vmatrix} \times \cdots \times \begin{vmatrix} \bar{\nu}_1^{F} & \bar{\xi}_{1,2}^{F} & \bar{\xi}_{1,3}^{F} \\ \bar{\xi}_{2,1}^{F} & \bar{\nu}_2^{F} & \bar{\xi}_{2,3}^{F} \\ \bar{\xi}_{3,1}^{F} & \bar{\xi}_{3,2}^{F} & \bar{\nu}_3^{F} \end{vmatrix}
\end{aligned} \tag{A8}
$$

$$
\begin{aligned}
P_{12}ABC &= \langle c_1^{B\dagger} c_2^{A\dagger} c_2^{B} c_1^{A} n_1^{A} \bar{n}_1^{B} \bar{n}_1^{C} \ldots \bar{n}_1^{F} \bar{n}_2^{A} n_2^{B} \bar{n}_2^{C} \ldots \bar{n}_2^{F} \bar{n}_3^{A} \bar{n}_3^{B} n_3^{C} \ldots \bar{n}_3^{F} \rangle \\
&= \langle c_1^{B\dagger} c_1^{A} \bar{n}_1^{C} \ldots \bar{n}_1^{F} c_2^{A\dagger} c_2^{B} \bar{n}_2^{A} n_2^{B} \bar{n}_2^{C} \ldots \bar{n}_2^{F} \bar{n}_3^{A} \bar{n}_3^{B} n_3^{C} \ldots \bar{n}_3^{F} \rangle \\
&= \langle c_1^{B\dagger} c_1^{A} \bar{n}_1^{C} \ldots \bar{n}_1^{F} c_2^{A\dagger} c_2^{B} \bar{n}_2^{C} \ldots \bar{n}_2^{F} \bar{n}_3^{A} \bar{n}_3^{B} n_3^{C} \ldots \bar{n}_3^{F} \rangle \\
&= \langle c_1^{A} c_2^{A\dagger} \bar{n}_3^{A} \rangle \langle c_1^{B\dagger} c_2^{B} \bar{n}_3^{B} \rangle \langle \bar{n}_1^{C} \bar{n}_2^{C} n_3^{C} \rangle \ldots \langle \bar{n}_1^{F} \bar{n}_2^{F} \bar{n}_3^{F} \rangle \\
&=? \begin{vmatrix} \bar{\xi}_{1,2}^{A} & \bar{\xi}_{1,3}^{A} \\ \xi_{2,3}^{A} & \nu_3^{A} \end{vmatrix} \times \begin{vmatrix} \xi_{1,2}^{B} & \xi_{1,3}^{B} \\ \bar{\xi}_{2,3}^{B} & \bar{\nu}_3^{B} \end{vmatrix} \times \begin{vmatrix} \bar{\nu}_1^{C} & \bar{\xi}_{1,2}^{C} & \bar{\xi}_{1,3}^{C} \\ \bar{\xi}_{2,1}^{C} & \bar{\nu}_2^{C} & \bar{\xi}_{2,3}^{C} \\ \xi_{3,1}^{C} & \xi_{3,2}^{C} & \nu_3^{C} \end{vmatrix} \times \cdots \times \begin{vmatrix} \bar{\nu}_1^{F} & \bar{\xi}_{1,2}^{F} & \bar{\xi}_{1,3}^{F} \\ \bar{\xi}_{2,1}^{F} & \bar{\nu}_2^{F} & \bar{\xi}_{2,3}^{F} \\ \bar{\xi}_{3,1}^{F} & \bar{\xi}_{3,2}^{F} & \bar{\nu}_3^{F} \end{vmatrix}
\end{aligned} \tag{A9}
$$
